# Supplementary material for: Robust Multimodal 3D Object Detection via Modality-Agnostic Decoding and Proximity-based Modality Ensemble
Source: arXiv:2407.19156 source file (2024-08-19)
Supplement: Supplementary file 1 [file X_suppl.tex]

\setcounter{table}{0}

\setcounter{figure}{0}

\appendix
% We provide a detailed PyTorch code of modality-agnostic decoding (MOAD) and proximity-based modality ensemble (PME) module in~\cref{supple:algorithm}.
In~\cref{supple:pme_analysis}, we compare modality ensemble strategies to validate the effectiveness of PME module.
Then, we provide additional qualitative results of MEFormer in~\cref{supple:qual} to further validate the effectiveness of PME in various environments.
\section{Analysis of PME}
\label{supple:pme_analysis}
\begin{table*}[t!]
\centering
\setlength{\tabcolsep}{20pt}
\begin{tabular}{lcc}
    \toprule
    Method & NDS & mAP \\
    % \midrule 
    \midrule
    Ours w/o PME & 73.66 & 71.25 \\
    % \midrule
    top-k ($k=300$) & 51.80 \scriptsize\textcolor{red}{($-21.86$)} & 33.34 \scriptsize\textcolor{red}{($-37.91$)} \\
    % NMS (IoU thres $=0.7$) & 61.59 & 52.43 \\
    NMS (IoU thres $=0.5$) & 63.86 \scriptsize\textcolor{red}{($-9.80$)} & 56.72 \scriptsize\textcolor{red}{($-14.53$)} \\
    % NMS (IoU thres $=0.3$) & 65.49 & 59.61 \\
    NME & 73.62 \scriptsize\textcolor{red}{($-0.04$)} & 71.15 \scriptsize\textcolor{red}{($-0.10$)} \\
    \midrule
    \textbf{PME} & \textbf{73.79} \scriptsize\textcolor{blue}{($+0.13$)} &\textbf{71.39} \scriptsize\textcolor{blue}{($+0.14$)} \\
    \bottomrule
\end{tabular}
\caption{
\textbf{Comparison of modality ensemble strategies.}
NME denotes naive modality ensemble which performs modality ensemble with no attention mask $M$ introduced in Eq. (9).
}
\label{ensemble_design}
\end{table*}

In this section, we compare various modality ensemble strategies to validate the effectiveness of the PME module for modality ensemble.
Results are shown in Table~\ref{ensemble_design}.
For top-k and NMS, we aggregate all box predictions from three modality decoding branches and apply these strategies based on confidence scores, and they show significant performance degradation compared to ours without PME.
In addition, NME that does not use proximity-based attention mask $M$ also shows a 0.1\% mAP drop compared to ours without PME while ours with PME shows 0.13\% NDS and 0.14\% mAP enhancement.
This verifies that adaptively aggregating box features from three modality decoding branches using PME is effective for box refinement.

% Our PME module improves the detection performance of MEFormer in all environments.
% Especially for objects in a middle distance, there is a 0.24\% performance improvement.
% Also, on a rainy day, there is a performance improvement of 0.16\%.
% These results validate that the PME module prevents noisy information transfer in challenging environments.
\section{More qualitative results}
\label{supple:qual}
\begin{figure*}
    \centering
    \includegraphics[width=0.95\textwidth]{supple/image/supple_qual_occluded.pdf}
    \caption{
    \textbf{Qualitative comparison of ours without PME and with PME.}
    Camera-only decoding branch fails to detect the pedestrian behind the traffic sign in the back left view camera.
    As a result, ours without PME misses the pedestrian due to the negative fusion, while ours with PME successfully localizes it.
    }
    \label{fig:supple_qual_occluded}
\end{figure*}
\begin{figure*}
    \centering
    \includegraphics[width=0.95\textwidth]{supple/image/supple_qual_dark.pdf}
    \caption{
    \textbf{Qualitative comparison of ours without PME and with PME.}
    Ours without PME fails to localize the motorcycle that the camera-only decoding branch identifies.
    However, ours with PME successfully localizes the motorcycle.
    }
    \label{fig:supple_qual_dark}
\end{figure*}
We validate the effectiveness of our PME module by comparing the qualitative results with and without PME.
In~\cref{fig:supple_qual_occluded}, the camera-only decoding branch fails to detect the pedestrian in the back left view camera since the traffic sign occludes the pedestrian.
As a result, ours without PME (\cref{fig:supple_qual_occluded}(a)) also misses the pedestrian due to the negative fusion problem.
However, ours with PME (\cref{fig:supple_qual_occluded}(b)) successfully detects the pedestrian by aggregating box features from the LiDAR decoding branch using PME module.
Additionally, from the front view camera in~\cref{fig:supple_qual_dark}, ours with PME (\cref{fig:supple_qual_dark}(b)) localizes the motorcycle, whereas without PME (\cref{fig:supple_qual_dark}(a)) fails to localize it even though the camera-only decoding branch detects it.
% Furthermore, in~\cref{fig:supple_qual2}, our framework without PME (\cref{fig:qual2_moad}) misclassifies the car in the back view camera as a truck.
% However, PME successfully classifies it as a car (\cref{fig:qual2_pme}).
These qualitative results show that the PME module prevents negative fusion during the modality fusion process.
% \clearpage
% {
%     \small
%     \bibliographystyle{ieeenat_fullname}
%     \bibliography{main}
% }

% \end{document}
