# Supplementary material for: Robust Multimodal 3D Object Detection via Modality-Agnostic Decoding and Proximity-based Modality Ensemble
Source: arXiv:2407.19156 source file (2024-08-19)
Supplement: Supplementary file 2 [file supple_qual_dark.tex]

\begin{figure*}
    \centering
    \includegraphics[width=0.95\textwidth]{supple/image/supple_qual_dark.pdf}
    \caption{
    \textbf{Qualitative comparison of ours without PME and with PME.}
    Ours without PME fails to localize the motorcycle that the camera-only decoding branch identifies.
    However, ours with PME successfully localizes the motorcycle.
    }
    \label{fig:supple_qual_dark}
\end{figure*}
