# Supplementary material for: Robust Multimodal 3D Object Detection via Modality-Agnostic Decoding and Proximity-based Modality Ensemble
Source: arXiv:2407.19156 source file (2024-08-19)
Supplement: Supplementary file 3 [file supple_qual_occluded.tex]

\begin{figure*}
    \centering
    \includegraphics[width=0.95\textwidth]{supple/image/supple_qual_occluded.pdf}
    \caption{
    \textbf{Qualitative comparison of ours without PME and with PME.}
    Camera-only decoding branch fails to detect the pedestrian behind the traffic sign in the back left view camera.
    As a result, ours without PME misses the pedestrian due to the negative fusion, while ours with PME successfully localizes it.
    }
    \label{fig:supple_qual_occluded}
\end{figure*}
