# Supplementary material for: Robust Multimodal 3D Object Detection via Modality-Agnostic Decoding and Proximity-based Modality Ensemble
Source: arXiv:2407.19156 source file (2024-08-19)
Supplement: Supplementary file 4 [file 0.tex]

% We provide a detailed PyTorch code of modality-agnostic decoding (MOAD) and proximity-based modality ensemble (PME) module in~\cref{supple:algorithm}.
In~\cref{supple:pme_analysis}, we compare modality ensemble strategies to validate the effectiveness of PME module.
Then, we provide additional qualitative results of MEFormer in~\cref{supple:qual} to further validate the effectiveness of PME in various environments.
