# Supplementary material for: Robust Multimodal 3D Object Detection via Modality-Agnostic Decoding and Proximity-based Modality Ensemble
Source: arXiv:2407.19156 source file (2024-08-19)
Supplement: Supplementary file 5 [file 1.tex]

\section{Algorithm}
\label{supple:algorithm}
