# Supplementary material for: Robust Multimodal 3D Object Detection via Modality-Agnostic Decoding and Proximity-based Modality Ensemble
Source: arXiv:2407.19156 source file (2024-08-19)
Supplement: Supplementary file 6 [file 2.tex]

\section{Analysis of PME}
\label{supple:pme_analysis}
\begin{table*}[t!]
\centering
\setlength{\tabcolsep}{20pt}
\begin{tabular}{lcc}
    \toprule
    Method & NDS & mAP \\
    % \midrule 
    \midrule
    Ours w/o PME & 73.66 & 71.25 \\
    % \midrule
    top-k ($k=300$) & 51.80 \scriptsize\textcolor{red}{($-21.86$)} & 33.34 \scriptsize\textcolor{red}{($-37.91$)} \\
    % NMS (IoU thres $=0.7$) & 61.59 & 52.43 \\
    NMS (IoU thres $=0.5$) & 63.86 \scriptsize\textcolor{red}{($-9.80$)} & 56.72 \scriptsize\textcolor{red}{($-14.53$)} \\
    % NMS (IoU thres $=0.3$) & 65.49 & 59.61 \\
    NME & 73.62 \scriptsize\textcolor{red}{($-0.04$)} & 71.15 \scriptsize\textcolor{red}{($-0.10$)} \\
    \midrule
    \textbf{PME} & \textbf{73.79} \scriptsize\textcolor{blue}{($+0.13$)} &\textbf{71.39} \scriptsize\textcolor{blue}{($+0.14$)} \\
    \bottomrule
\end{tabular}
\caption{
\textbf{Comparison of modality ensemble strategies.}
NME denotes naive modality ensemble which performs modality ensemble with no attention mask $M$ introduced in Eq. (9).
}
\label{ensemble_design}
\end{table*}

In this section, we compare various modality ensemble strategies to validate the effectiveness of the PME module for modality ensemble.
Results are shown in Table~\ref{ensemble_design}.
For top-k and NMS, we aggregate all box predictions from three modality decoding branches and apply these strategies based on confidence scores, and they show significant performance degradation compared to ours without PME.
In addition, NME that does not use proximity-based attention mask $M$ also shows a 0.1\% mAP drop compared to ours without PME while ours with PME shows 0.13\% NDS and 0.14\% mAP enhancement.
This verifies that adaptively aggregating box features from three modality decoding branches using PME is effective for box refinement.

% Our PME module improves the detection performance of MEFormer in all environments.
% Especially for objects in a middle distance, there is a 0.24\% performance improvement.
% Also, on a rainy day, there is a performance improvement of 0.16\%.
% These results validate that the PME module prevents noisy information transfer in challenging environments.
