# Supplementary material for: Robust Multimodal 3D Object Detection via Modality-Agnostic Decoding and Proximity-based Modality Ensemble
Source: arXiv:2407.19156 source file (2024-08-19)
Supplement: Supplementary file 7 [file 3.tex]

\section{More qualitative results}
\label{supple:qual}
\begin{figure*}
    \centering
    \includegraphics[width=0.95\textwidth]{supple/image/supple_qual_occluded.pdf}
    \caption{
    \textbf{Qualitative comparison of ours without PME and with PME.}
    Camera-only decoding branch fails to detect the pedestrian behind the traffic sign in the back left view camera.
    As a result, ours without PME misses the pedestrian due to the negative fusion, while ours with PME successfully localizes it.
    }
    \label{fig:supple_qual_occluded}
\end{figure*}
\begin{figure*}
    \centering
    \includegraphics[width=0.95\textwidth]{supple/image/supple_qual_dark.pdf}
    \caption{
    \textbf{Qualitative comparison of ours without PME and with PME.}
    Ours without PME fails to localize the motorcycle that the camera-only decoding branch identifies.
    However, ours with PME successfully localizes the motorcycle.
    }
    \label{fig:supple_qual_dark}
\end{figure*}
We validate the effectiveness of our PME module by comparing the qualitative results with and without PME.
In~\cref{fig:supple_qual_occluded}, the camera-only decoding branch fails to detect the pedestrian in the back left view camera since the traffic sign occludes the pedestrian.
As a result, ours without PME (\cref{fig:supple_qual_occluded}(a)) also misses the pedestrian due to the negative fusion problem.
However, ours with PME (\cref{fig:supple_qual_occluded}(b)) successfully detects the pedestrian by aggregating box features from the LiDAR decoding branch using PME module.
Additionally, from the front view camera in~\cref{fig:supple_qual_dark}, ours with PME (\cref{fig:supple_qual_dark}(b)) localizes the motorcycle, whereas without PME (\cref{fig:supple_qual_dark}(a)) fails to localize it even though the camera-only decoding branch detects it.
% Furthermore, in~\cref{fig:supple_qual2}, our framework without PME (\cref{fig:qual2_moad}) misclassifies the car in the back view camera as a truck.
% However, PME successfully classifies it as a car (\cref{fig:qual2_pme}).
These qualitative results show that the PME module prevents negative fusion during the modality fusion process.
