# Supplementary material for: Robust Multimodal 3D Object Detection via Modality-Agnostic Decoding and Proximity-based Modality Ensemble
Source: arXiv:2407.19156 source file (2024-08-19)
Supplement: Supplementary file 8 [file ensemble_design.tex]

\begin{table*}[t!]
\centering
\setlength{\tabcolsep}{20pt}
\begin{tabular}{lcc}
    \toprule
    Method & NDS & mAP \\
    % \midrule 
    \midrule
    Ours w/o PME & 73.66 & 71.25 \\
    % \midrule
    top-k ($k=300$) & 51.80 \scriptsize\textcolor{red}{($-21.86$)} & 33.34 \scriptsize\textcolor{red}{($-37.91$)} \\
    % NMS (IoU thres $=0.7$) & 61.59 & 52.43 \\
    NMS (IoU thres $=0.5$) & 63.86 \scriptsize\textcolor{red}{($-9.80$)} & 56.72 \scriptsize\textcolor{red}{($-14.53$)} \\
    % NMS (IoU thres $=0.3$) & 65.49 & 59.61 \\
    NME & 73.62 \scriptsize\textcolor{red}{($-0.04$)} & 71.15 \scriptsize\textcolor{red}{($-0.10$)} \\
    \midrule
    \textbf{PME} & \textbf{73.79} \scriptsize\textcolor{blue}{($+0.13$)} &\textbf{71.39} \scriptsize\textcolor{blue}{($+0.14$)} \\
    \bottomrule
\end{tabular}
\caption{
\textbf{Comparison of modality ensemble strategies.}
NME denotes naive modality ensemble which performs modality ensemble with no attention mask $M$ introduced in Eq. (9).
}
\label{ensemble_design}
\end{table*}
