# Supplementary material for: Robust Multimodal 3D Object Detection via Modality-Agnostic Decoding and Proximity-based Modality Ensemble
Source: arXiv:2407.19156 source file (2024-08-19)
Supplement: Supplementary file 13 [file sensor_malfunction.tex]

\begin{table}[ht]
\centering
\caption{Robustness against noisy point clouds}
% \label{lidar_sparsity}
\begin{tabular}{lccccc}
    \toprule
    Method & Modality & 16-beam & 8-beam & 4-beam& 1-beam\\
    \midrule 
    \midrule
    Transfusion-L$^\ast$ & L & 58.9 & & 49.6 & 22.2 \\
    BEVFusion$^\ast$ & L+C & 63.0 & & 55.3 & 30.4 \\
    DeepInteraction & L+C & 61.0 & & 55.1 & 27.2 \\
    SparseFusion & L+C & 65.5 & & 59.9 & 33.5 \\
    CMT & L+C & 67.6 & & 62.2 & 43.4 \\
    \midrule
    Ours w/o PME & L+C & 68.2 &-  & 62.8 & - \\
    \textbf{Ours} & L+C &\textbf{68.9} & \textbf{-} & \textbf{63.3} & \textbf{41.6} \\
    \bottomrule
\end{tabular}
\end{table}
