# Supplementary material for: Robust Multimodal 3D Object Detection via Modality-Agnostic Decoding and Proximity-based Modality Ensemble
Source: arXiv:2407.19156 source file (2024-08-19)
Supplement: Supplementary file 14 [file 4_tmp.tex]

\input{supple/table/sensor_malfunction}
